# Supplementary material for: Co-optimization of Short- and Long-term Decisions for the Transmission Grid's Resilience to Flooding
Source: arXiv:2503.06909 source file (2025-03-10)
Supplement: Supplementary file 1 [file appendix.tex]

\section{Supplementary Material}
\begin{figure*}[h]
  \centering
  \includegraphics[width=\textwidth]{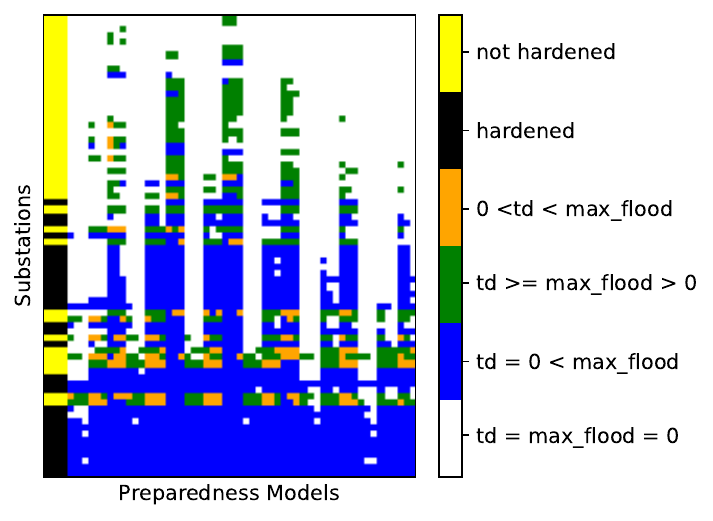} % Adjust the width and file name as needed
  \caption{Your figure caption here.}
  \label{fig:your_label}
\end{figure*}
\begin{figure*}
  \centering

  \subfloat[Caption for Figure a\label{fig:subfig-a}]{\includegraphics[width=0.3\textwidth]{solution_figs/granular_voll_500.pdf}}\hfill
  \subfloat[Caption for Figure b\label{fig:subfig-b}]{\includegraphics[width=0.3\textwidth]{solution_figs/granular_voll_500.pdf}}\hfill \subfloat[Caption for Figure c\label{fig:subfig-c}]{\includegraphics[width=0.3\textwidth]{solution_figs/granular_voll_500.pdf}}

  \caption{Overall caption for the three sub figures.}
  \label{fig:overall_label}
\end{figure*}

\begin{figure}[h]
    \centering
    \includegraphics[width=0.5\textwidth]{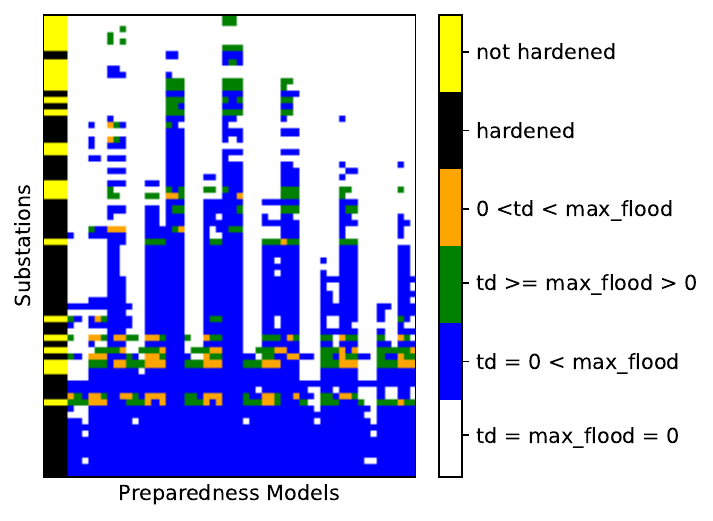}
    \captionof{figure}{Decoupled Decision making for VOLL = 250}
    \label{fig:scenario_tree}
\end{figure}

\begin{figure}[h]
    \centering
    \includegraphics[width=0.5\textwidth]{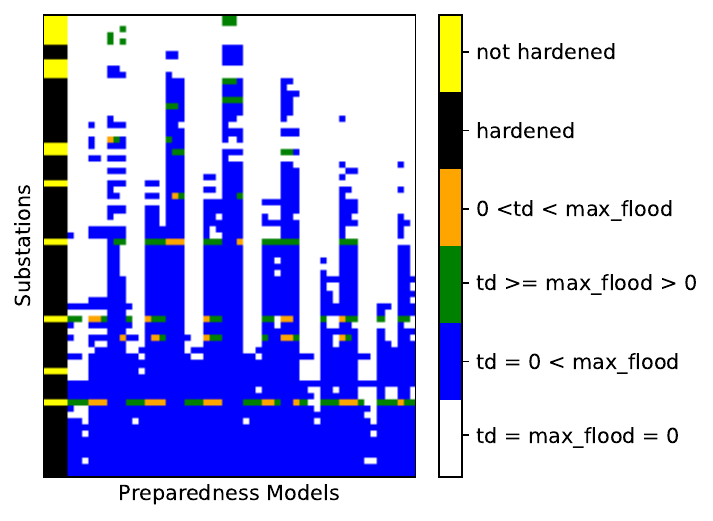}
    \captionof{figure}{Decoupled Decision making for VOLL = 500}
    \label{fig:scenario_tree}
\end{figure}

\begin{figure}[h]
    \centering
    \includegraphics[width=0.5\textwidth]{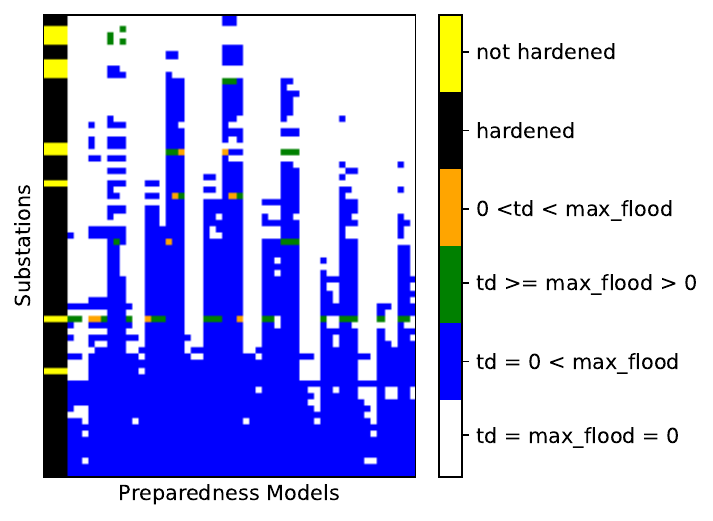}
    \captionof{figure}{Decoupled Decision making for VOLL = 1000}
    \label{fig:scenario_tree}
\end{figure}

\begin{figure}[h]
    \centering
    \includegraphics[width=0.5\textwidth]{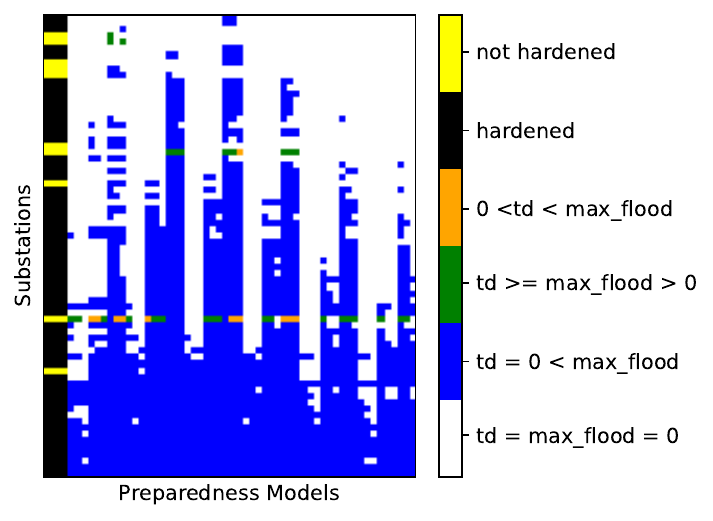}
    \captionof{figure}{Decoupled Decision making for VOLL = 2000}
    \label{fig:scenario_tree}
\end{figure}

\begin{figure}[h]
    \centering
    \includegraphics[width=0.5\textwidth]{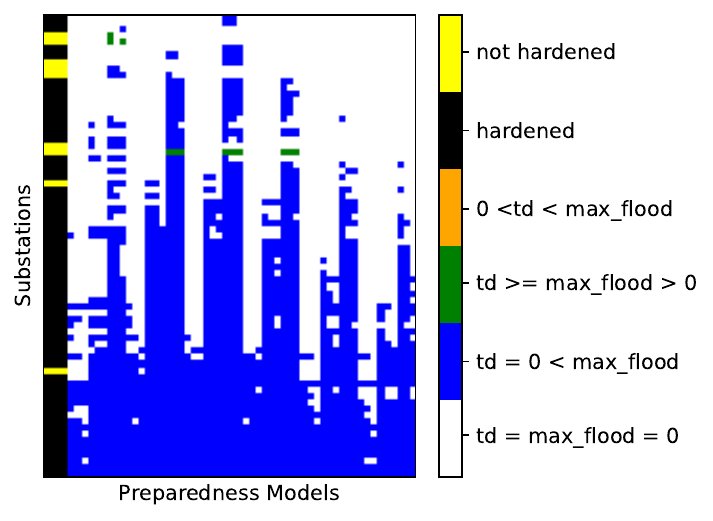}
    \captionof{figure}{Decoupled Decision making for VOLL = 3000}
    \label{fig:scenario_tree}
\end{figure}

\begin{figure}[h]
    \centering
    \includegraphics[width=0.5\textwidth]{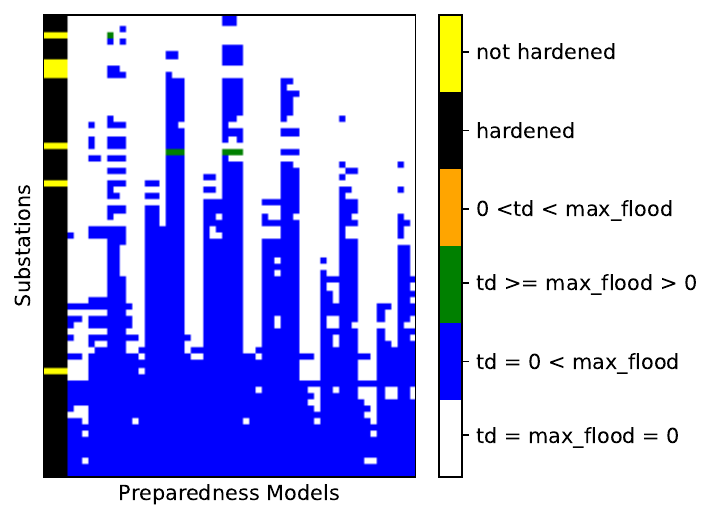}
    \captionof{figure}{Decoupled Decision making for VOLL = 4000}
    \label{fig:scenario_tree}
\end{figure}

\begin{figure}[h]
    \centering
    \includegraphics[width=0.5\textwidth]{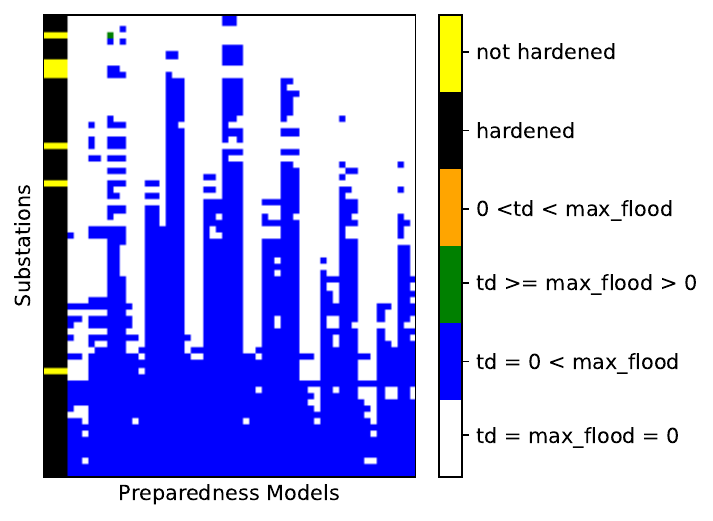}
    \captionof{figure}{Decoupled Decision making for VOLL = 5000}
    \label{fig:scenario_tree}
\end{figure}

\begin{figure}[h]
    \centering
    \includegraphics[width=0.5\textwidth]{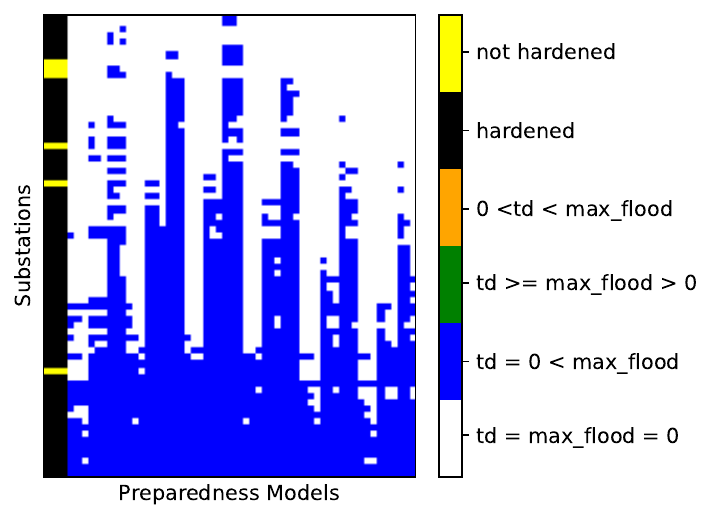}
    \captionof{figure}{Decoupled Decision making for VOLL = 6000}
    \label{fig:scenario_tree}
\end{figure}

\begin{figure}[h]
    \centering
    \includegraphics[width=0.5\textwidth]{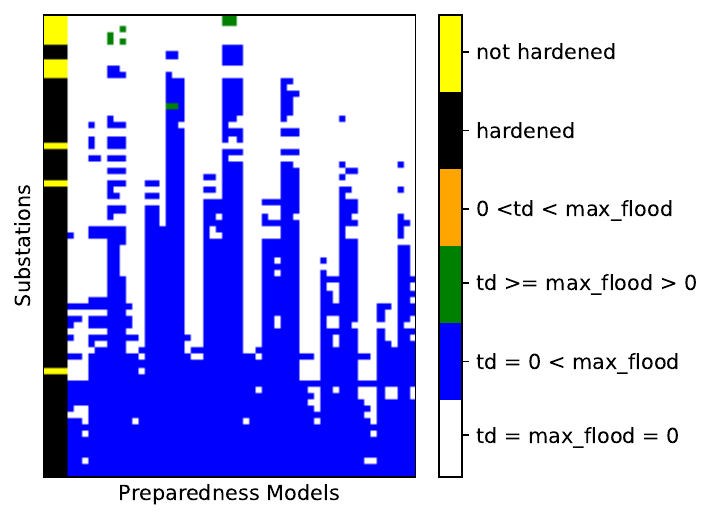}
    \captionof{figure}{Coupled Decision making for v = 25k}
    \label{fig:scenario_tree}
\end{figure}

\begin{figure}[h]
    \centering
    \includegraphics[width=0.5\textwidth]{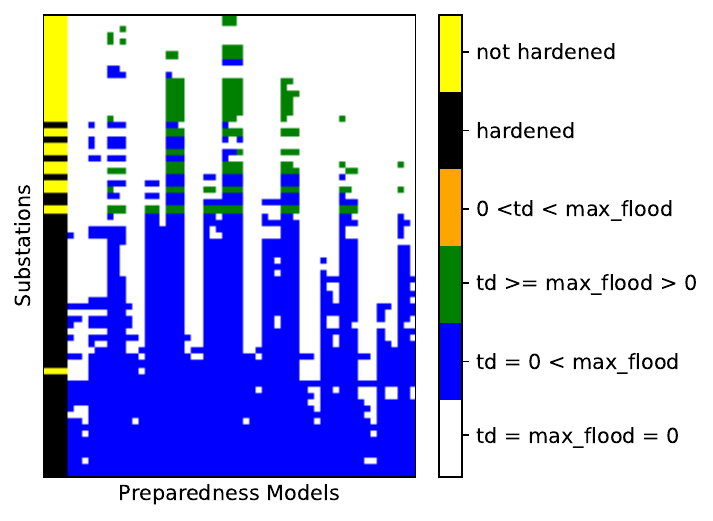}
    \captionof{figure}{Coupled Decision making for v = 50k}
    \label{fig:scenario_tree}
\end{figure}

\begin{figure}[h]
    \centering
    \includegraphics[width=0.5\textwidth]{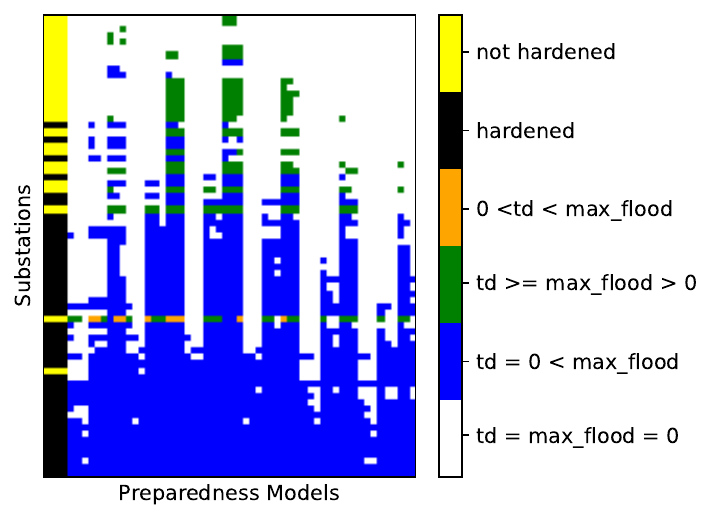}
    \captionof{figure}{Coupled Decision making for v = 75k}
    \label{fig:scenario_tree}
\end{figure}
